# Supplementary material for: Efficient Sensorimotor Learning for Open-world Robot Manipulation
Source: arXiv:2505.06136 source file (2025-05-07)
Supplement: Supplementary file 1 [file lotus_appendix.tex]

\section{\lotus{} Implementation Details}
\label{sec:lotus:implementation}
